# Supplementary material for: Low Latency Transformer Inference on FPGAs for Physics Applications with hls4ml
Source: arXiv:2409.05207 source file (2024-09-08)
Supplement: Supplementary file 1 [file adaeappendix.tex]

\section{Artifact Description / Artifact Evaluation Appendix}
